# Supplementary material for: Iterative Translation Refinement with Large Language Models
Source: arXiv:2306.03856 source file (2024-05-01)
Supplement: Supplementary file 1 [file table_automatic_results_gpt_appendix.tex]

\small
\setlength{\tabcolsep}{0.4ex}
\begin{tabular}{lcccccccccccccc}
\toprule
& \multicolumn{2}{c}{\scriptsize{WMT21} \small de$\rightarrow$en} 
& \multicolumn{2}{c}{\scriptsize{WMT21} \small en$\rightarrow$de} 
& \multicolumn{2}{c}{\scriptsize{WMT21} \small zh$\rightarrow$en} 
& \multicolumn{2}{c}{\scriptsize{WMT21} \small en$\rightarrow$zh} 
& \multicolumn{2}{c}{\scriptsize{WMT22} \small de$\rightarrow$fr} 
& \multicolumn{2}{c}{\scriptsize{WMT22} \small en$\rightarrow$ja} 
& \multicolumn{2}{c}{\scriptsize{WMT22} \small uk$\rightarrow$cs} \\
\cmidrule(lr){2-3}\cmidrule(lr){4-5}\cmidrule(lr){6-7}\cmidrule(lr){8-9}\cmidrule(lr){10-11}\cmidrule(lr){12-13}\cmidrule(lr){14-15}
& \scriptsize{chrF++} & \tiny{COMET\textsubscript{DA}} & \scriptsize{chrF++} & \tiny{COMET\textsubscript{DA}} & \scriptsize{chrF++} & \tiny{COMET\textsubscript{DA}} & \scriptsize{chrF++} & \tiny{COMET\textsubscript{DA}} & \scriptsize{chrF++} & \tiny{COMET\textsubscript{DA}} & \scriptsize{chrF++} & \tiny{COMET\textsubscript{DA}} & \scriptsize{chrF++} & \tiny{COMET\textsubscript{DA}} \\
\midrule
Reference\textsubscript{A} & - & - & - & - & - & - & - & - & - & - & - & - & - & -  \\
\cdashlinelr{1-15}
Translate & \textbf{57.55} & \textbf{.8606} & \textbf{53.54} & .8427 & \textbf{53.74} & .8199 & \textbf{20.61} & .8300 & \textbf{59.50} & \textbf{.8395} & 25.89 & .8863 & \textbf{54.64} & \textbf{.9074} \\
Refine & 51.91 & .8525 & 50.57 & \textbf{.8478} & 49.06 & .8156 & 19.28 & \textbf{.8417} & 55.83 & .8353 & \textbf{27.30} & \textbf{.8941} & 53.06 & .9040 \\
Refine\textsubscript{Contrast} & 52.47 & .8452 & 51.21 & .8211 & 51.77 & \textbf{.8538} & 19.69 & .8395 & 56.37 & .8308 & 26.71 & .8928 & 54.29 & .9036 \\
Refine\textsubscript{Random} & 51.79 & .7777 & 46.56 & .7906 & 47.11 & .8323 & 17.49 & .8126 & - & - & - & - & - & - \\
Paraphrase & 40.05 & .8044 & 43.54 & .8197 & 40.92 & .7931 & 17.14 & .8144 & 44.28 & .7937 & 23.18 & .8592 & 40.04 & .8625 \\
\bottomrule
\end{tabular}
